# Supplementary material for: Symmetric Uncertainty-Aware Feature Transmission for Depth Super-Resolution
Source: arXiv:2306.00386 source file (2023-06-01)
Supplement: Supplementary file 1 [file fig_supplement_nyu.pdf]

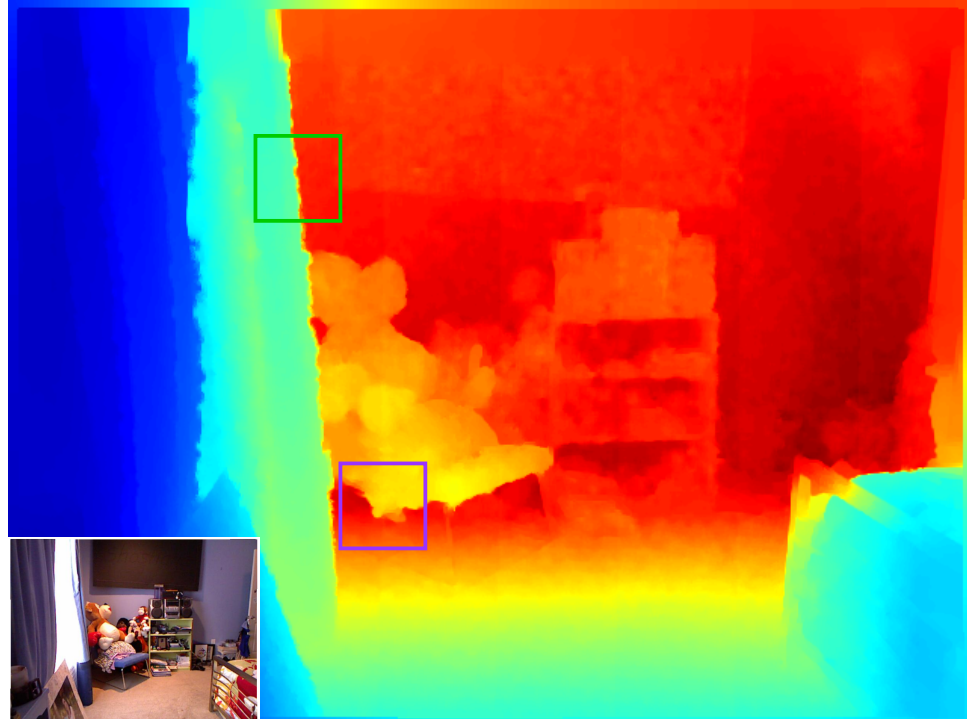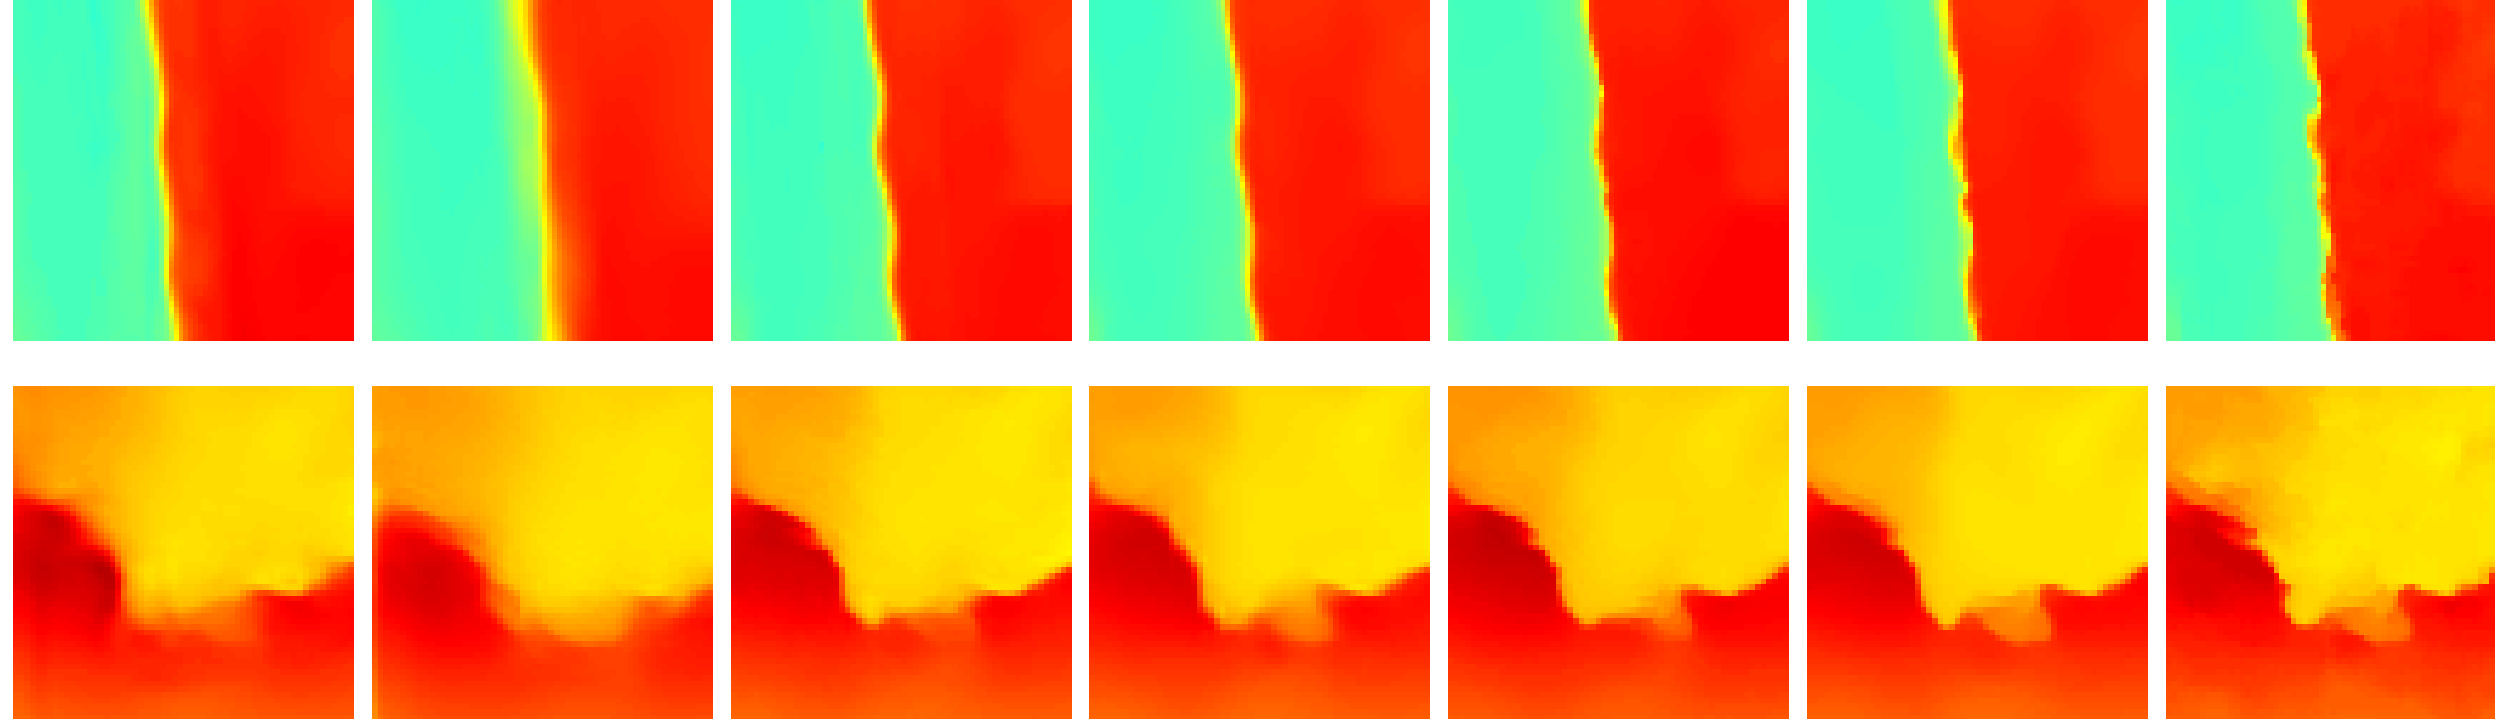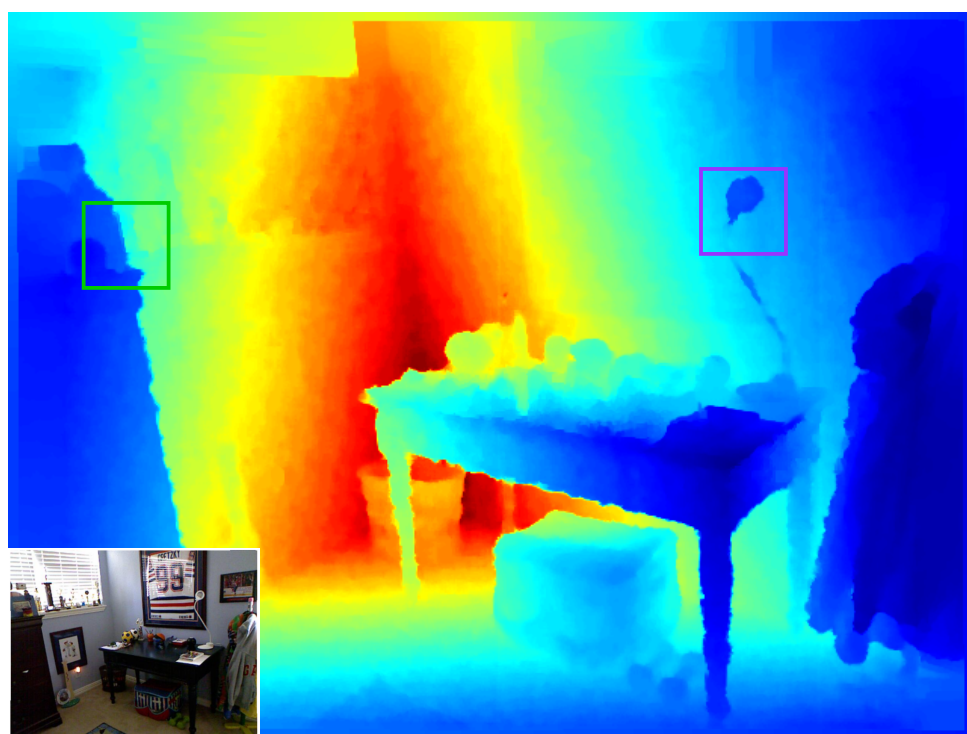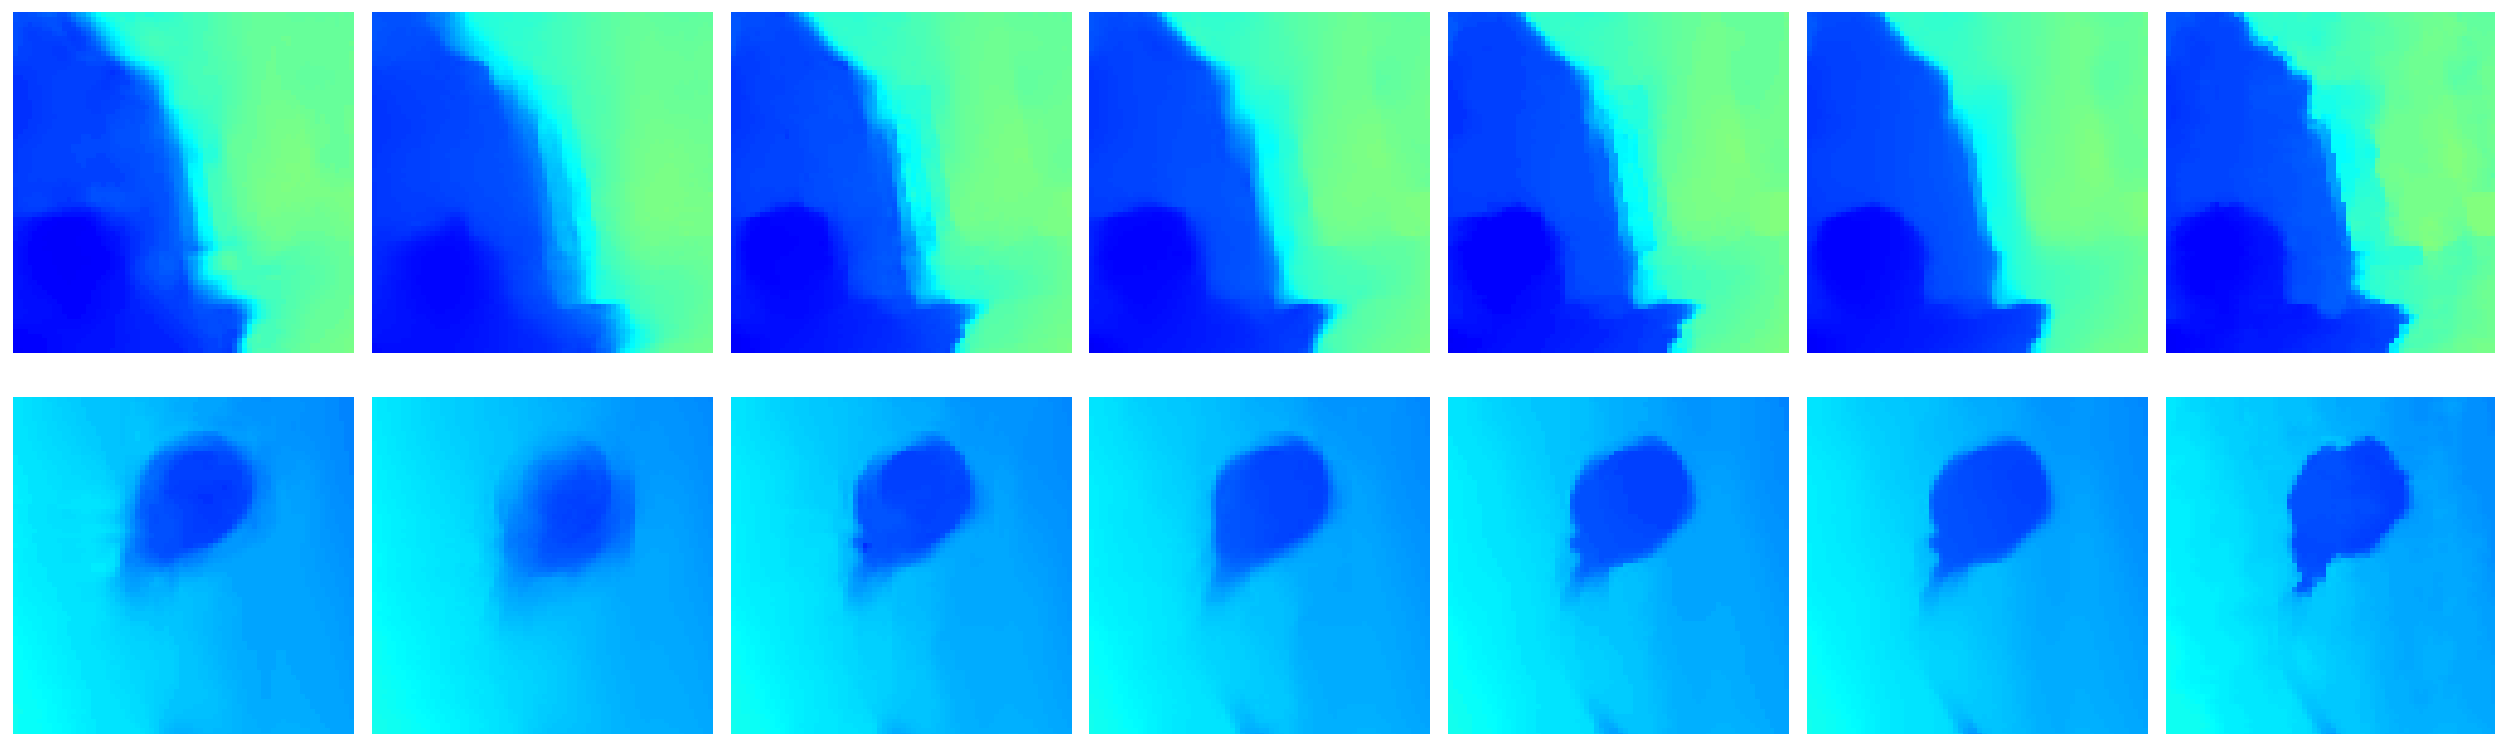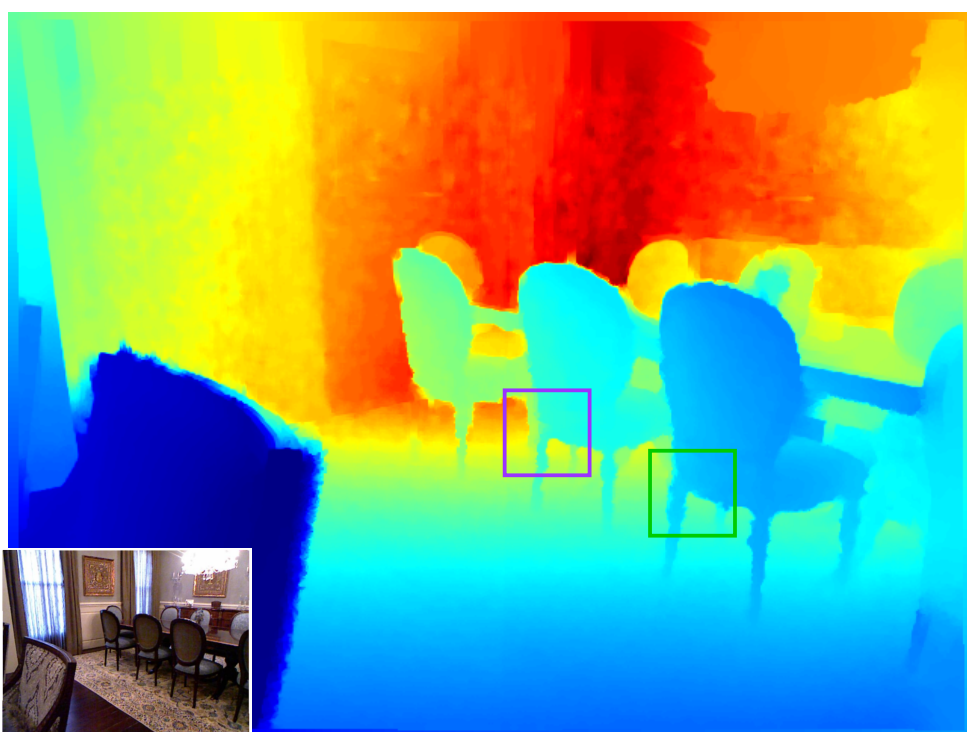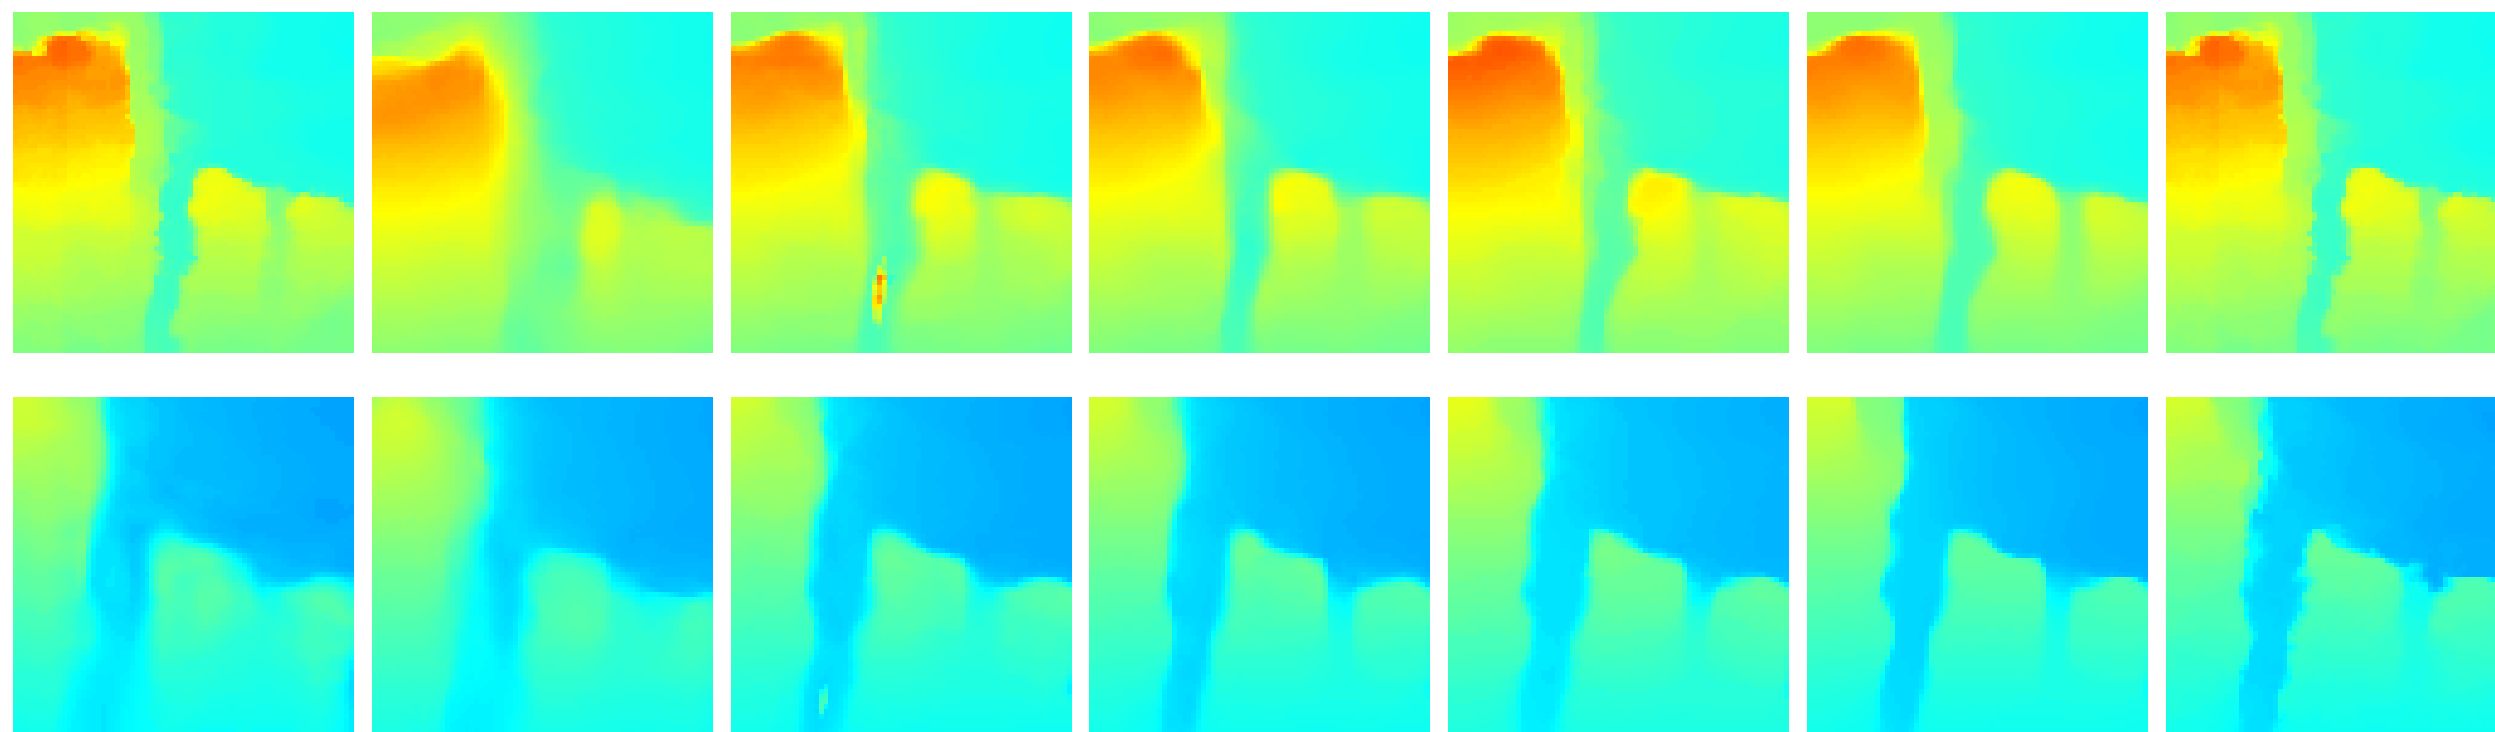

(a) Ground truth depth map and color image

(b) DJF

(c) SVLRM

(d) DKN

(e) FDSR

(f) JIIF

(g) SUFT

(h) GT
